# Supplementary material for: Applied Choreographies
Source: arXiv:1510.03637 source file (2020-12-14)
Supplement: Supplementary file 1 [file additional_material.tex]

%auto-ignore
\section{Applied Choreographies}

\begin{figure*}
{\footnotesize
\begin{displaymath}
\hspace{-5pt}\begin{array}{c}
\infer[\did{C}{Send}]
{
	\env,\ \eta; C
	\quad \to\quad
	\env',\ C
}{
	\eta = \gensend
	&
	\renv{\env}{\eta}{\env'}
}
\quad
\infer[\did{C}{Recv}]
{
	\env,\ \genbranchI
	\quad \to\quad
	\env',\ C_j
}{
	j \in I
	&
	\renv{\env}{\com{k}{\role A}{\pid q[\role B].o_j(x_j)}}{\env'}
}
\\[5pt]
\infer[\did{C}{Com}]
{
	\env,\ \eta; C
	\to
	\env',\ \genrecv;C
}{
	\eta = \gencom
	% \\[1pt]
	&
	\renv{\env}{\gensend}{\env'}
}
% \quad
% \infer[\did{C}{Cond}]
% {
% 	\env,\ \cond{\pid p.e}{C_1}{C_2}
% 	\quad\to\quad
% 	\env,\ C_i
% }
% {
% 	i = 1 \text{ if } \evalfn(e, \env(\pid p).\estate) = \text{ true, }
% 	i = 2 \text{ otherwise}
% }
% \\[5pt]
% \infer[\did{C}{Ctx}]
% {
% 	\env, \recDef{X}{C_2}{C_1} \to
% 	\env^\prime, \recDef{X}{C_2}{C^\prime_1}
% }
% {
% 	\env, C_1 \to \env^\prime, C^\prime_1
% }
\quad
\infer[\did{C}{Eq}]
{
	\env, C_1 \to \env^\prime, C_2
}
{
	\ctx{R} \in \{\,\equiv\,,\,\swapC\,\}
	&
	C_1 \,\ctx{R}\, C^\prime_1
	\\[1pt]
	\env, C^\prime_1 \to \env^\prime, C^\prime_2
	&
	C^\prime_2 \,\ctx{R}\, C_2
}
\\[5pt]
\infer[\did{C}{Start}]
{
	\env,\ \genstart; C
	\to
	\env',\
	C[k'/k][\pids r/\pids q] 
}
{
	\env\fresh{k',\pids r}
% 	&
% 	\fresh{k'}
% 	&
% 	\pid p \in \env(l)
	&
	\delta = \deltastart{k'}{l.\prc pA, \wtil{l.\prc rB}}
	% \eta[k'/k][\pids r/\pids q]
	&
	\renv{\env}{\delta}{\env'}
}
% \infer[\did{C}{Par}]
% {
% 	\env, C_1\pp C_2
% 	\to
% 	\env', C'_1 \pp C_2
% }
% {
% 	\env, C_1
% 	\to
% 	\env', C'_1
% }
% \quad
% \\[5pt]
% \infer[\did{C}{PStart}]
% {
% 	\begin{array}{c}
% 	\env,
% 	\req{k}{\pid p[\role A]}
% 	{\wtil{l.\role B}}; C
% 	\pp
% 	\prod_i
% 	\big(
% 	\genacci; C_i
% 	\big)
% 	\to
% 	\\ \qquad
% 	\env',\ 
% 	C[k'/k] \pp \prod_i\big(\ C_i[k'/k][\pids r_i /\pids q_i] \ \big)
% 	\pp
% 	\prod_i
% 	\big(
% 	\genacci; C_i
% 	\big)
% 	\end{array}
% }
% {
% 	\begin{array}c
% 	i \in \{1,\dots,n\}
% 	\quad
% 	\fresh{k'}
% 	\quad
% 	\{ \wtil{l.\role B} \} = \biguplus_i \{\wtil{l_i.\role B_i}\}
% 	\quad
% 	\fresh{\pids r}
% 	\\[2pt]
% 	\{\pids r\} = \bigcup_i \{ \pids r_i \}
% 	\quad
% 	\pid p \in \env(l)
% 	\quad
% 	\delta = \deltastart{k'}{l.\pid p[\role A],\wtil{l_1.\pid r_1[\role
% 	B_1]},\dots,\wtil{l_n.\pid r_n[\role B_n]}}
% 	\quad
% 	\renv{\env}{\delta}{\env'}
% 	\end{array}
% }
\end{array}
\end{displaymath}}
\vspace{-1em}
\caption{Applied Choreographies, semantics (selected).}
\label{fig:cc_semantics_sos}
\end{figure*}

\input{applied_choreographies/figures/chor_swap}

\newpage

\section{Typing}

In addition to the description in \cref{sec:typing} we comment the additional
rules in \cref{fig:typing_rules_full}. 

In Rule $\did{T}{End}$ $\end$ holds if the protocols for all sessions have
terminated (i.e., all local typings have type $\gend$). In Rule $\did{T}{Def}$
the condition $\Gamma' |_{\locs} \subseteq \Gamma$ checks that the body of
the recursive procedure does not introduce unexpected services
($\Gamma'|_{\locs}$ returns all service typings in $\Gamma'$).

\input{applied_choreographies/figures/chor_typing_rules_full}

\newpage

\begin{figure}
{$$
\begin{array}c
	\infer[\did{GS}{ComCom}]{
	\begin{array}{l}
		\gcom{\role A}{\role B}{\{\op{o}_i(U_i);\gcom{\role C}{\role
			D}{\{\op{o}_j'(U_j');G_{ij}\}_{j \in J}}\}_{i \in I}}
		\\\hspace{.3\textwidth}
		\swapG \quad
		\gcom{\role C}{\role D}{\{\op{o}_j'(U_j');\gcom{\role A}{\role
			B}{\{\op{o}_i(U_i);G_{ij}\}_{i \in I}}\}_{j \in J}}
	\end{array}
}
{	\{\role A, \role B\} \cap \{\role C, \role D\} = \emptyset }
\\[20pt]
\infer[\did{GS}{ComRecv}]{
	\begin{array}c
	\gcom{\role A}{\role B}{\{\op{o}_i(U_i);\grecv{\role C}{\role D}{\op{o}(U)};G_i\}}
	\quad \swapG \quad
	\grecv{\role C}{\role D}{\op{o}(U)};\gcom{\role A}{\role B}{\{\op{o}_i(U_i);G_i\}}
	\end{array}
}
{	
	\{\role A, \role B\}  \cap \{\role D\} = \emptyset
 }
\\[15pt]
\infer[\did{GS}{RecvRecv}]{
	\begin{array}c
	\grecv{\role A}{\role B}{\op{o}(U)};\grecv{\role C}{\role D}{\op{o}'(U)};G
	\quad \swapG \quad
	\grecv{\role C}{\role D}{\op{o}'(U)};\grecv{\role A}{\role B}{\op{o}(U)};G
	\end{array}
}{
	\role B \neq \role D
}
\end{array}
$$}
	\caption{Global types --- Swap Relation $\swapG$.}
	\label{fig:cc_global_types_swap}
\end{figure}

\input{applied_choreographies/figures/chor_typing_buffer}

\newpage

% \subsubsection{Typing Example}

% \input{applied_choreographies/examples/typing_example}

% \newpage

\section{Endpoint Projection}
We report the complete definition of choreography annotation, process
projection, merging function, and grouping function, respectively in
\cref{fig:cc_annotation}, \cref{fig:cc_projection},
\cref{fig:merging_function}, and \cref{fig:grouping}.

\begin{figure}
$$\begin{array}{rcl}
			@C & = & \emptyset@C \hfill
			\\\\
			d@C & = & \begin{cases}
				\eta ; d@C'								& \mbox{if } C = \eta ; C'
				\\
				d@C_1 \pp d@C_2 					& \mbox{if } C = C_1 | C_2
				\\
				\com{k}{\role A}{\pid q[\role B].\{o_i(x_i);d@C_i)\}_{i \in I}}
																						& \mbox{if } C = \genbranchI
				\\
				\recDef{X\carr{\pids p}}{d'@C''}{d'@C'}
																						& \mbox{if } 
																							\begin{array}l
																							C = \recDef{X}{C''}{C'} 
																							\ \wedge \
																							\\
																							\pids p = \fp(C'')
																							\ \wedge \
																							d' = d \cup 
																								(X,X\carr{\pids p})	
																							\end{array}

				\\
				\genacc ; d@C' 											&	\mbox{if } C = \genacc ; C'	
				\\
				\cond{\pid p.e}{d@C_1}{d@C_2}
																						& \mbox{if } 
																							C = \cond{\pid p.e}{C_1}{C_2}
				\\
				\recCall{X\carr{\pids p}} 					&	\mbox{if } C = X
																							\ \wedge \ 
																							(X,X\carr{\pids p}) \in d
				\\
				\inact															& \mbox{if } C = \inact
			\end{cases}
\end{array}$$
	\caption{Choreography Calculus --- Annotation operator}
	\label{fig:cc_annotation}
\end{figure}

\section{Dynamic Correlation Calculus}

\begin{figure}
\small\begin{displaymath}
\hspace{-5pt}\setlength\arraycolsep{2.5pt}\begin{array}{llll}
	\did{DCC}{Recv}
	&
	t_c = \evalfn(e, t)
	\ \wedge \
	M( t_c ) = ( o, t' ) :: \til m
	& \Rightarrow &
	\jprc{\oneway{o}{x} \qfrom{e};B}{t}{M}
	\to
	\jprc{B}{t \tcopy{x}{t'} }{M[t_c \mapsto \til m]}
	\\[2pt]
	\did{DCC}{Cq} 
	&
	\begin{array}l
		P = \jprc{\cq{x};B}{t}{M}
		\\
		\wedge \ t_c \not \in \bigcup_i \dom(M_i) \cup \m{dom}(M)
	\end{array}
	& \Rightarrow &
		\begin{array}l
		\jsrv{B_s,\ P \pp \prod_i \jprc{B_i}{t_i}{M_i}}l
			\to \\ \quad 
		\jsrv{B_s,\ \jprc{B}{t \tcopy{x}{t_c}}{M[t_c \mapsto \emptyseq]}
			\pp \prod_i \jprc{B_i}{t_i}{M_i}}l
		\end{array}
	\\[10pt]
	\did{DCC}{Send} 
	&
	\begin{array}{l}
		P = \jprc{\notify{o}{e_1}{e_2} \qto e_3; B}{t}{M}
		\\
		\wedge \ \evalfn( e_1, t ) = l'
		\ \wedge \
		\evalfn( e_3, t ) = t_c
		\\
		\wedge \ \evalfn(	e_2, t ) = t_m
		\\
		\wedge \ M'' = M'[t_c \mapsto M'(t_c) :: (o, t_m )]
	\end{array}
	& \Rightarrow &
	\begin{array}l
		\jsrv{B_s, P \pp P_1 }{l} \pp 
			\jsrv{B_s', \jprc{B'}{t'}{M'} \pp P_2}{l'}
		\to \\[2pt] \quad 
		 \jsrv{B_s, \jprc{B}{t}{M} \pp P_1 }{l} \pp 
			\jsrv{B_s', \jprc{B'}{t'}{M''} \pp P_2}{l'}
	\end{array}
	\\[20pt]
	\did{DCC}{Start}
	&
	\begin{array}l
		P_1 = \jprc{\notify{?}{e_1}{e_2};B_1}{t_1}{M_1}
		\\
		\wedge \ \evalfn( e_1, t_1 ) = l
		\\
		\wedge \ Q = \jprc{B}{t_\bot\tcopy{x}{\evalfn( e_2, t_1 )} }{\emptyset}
	\end{array}
	& \Rightarrow &
	\begin{array}l
		\jsrv{!(x);B,\ P}{l}	\pp	\jsrv{B'_s,\ P_1 \pp P_2}{l'}
		 \to \\[2pt] \quad \jsrv{!(x);B,\ Q \pp P}{l}
			\pp \jsrv{B'_s,\ \jprc{B_1}{t_1}{M_1} \pp P_2}{l'}	
		\end{array}
\end{array}
\end{displaymath}
	\vspace{-1em}
	\caption{Dynamic Correlation Calculus, semantics (selected).}
	\label{fig:js_semantics_sos}
\end{figure}

\begin{figure}[h]
% $$
% 	\hspace{-1em}\begin{array}{c}
% 		\recDef{X}{B'}{B[X]}
% 		\equiv
% 		\recDef{X}{B'}{B[B']}
% 		\\[.5em]
% 		P \equiv P \pp \jprc{\inact}{t}{\emptyset}
% 		\qquad
% 		(P_1 \pp P_2) \pp P_3  \equiv P_1 \pp (P_2 \pp P_3)
% 		\\[.5em]
% 		P \pp P^\prime \equiv P^\prime \pp P 
% 		\qquad
% 		% \jsrv{B_s, P \pp P'}l \equiv \jsrv{B_s, P' \pp P}l
% 		S \pp S^\prime \equiv S^\prime \pp S 
% 		\\[.5em]
% 		(S_1 \pp S_2) \pp S_3  \equiv S_1 \pp (S_2 \pp S_3)
% 	\end{array}
% $$
{\footnotesize$$
	\hspace{-1em}\begin{array}{c}
		\jprc{\recDef{X}{B'}{B[X]}}{t}{M}
		\equiv
		\jprc{\recDef{X}{B'}{B[B']}}{t}{M}
		\\[.5em]
		P \equiv P \pp \jprc{\inact}{t}{\emptyset}
		\qquad
		(P_1 \pp P_2) \pp P_3 \equiv P_1 \pp (P_2 \pp P_3)
		\\[.5em]
		P \pp P' \equiv P' \pp P
		\qquad
		% \jsrv{B_s, P \pp P'}l \equiv \jsrv{B_s, P' \pp P}l
		S \pp S^\prime \equiv S^\prime \pp S 
		\\[.5em]
		(S_1 \pp S_2) \pp S_3  \equiv S_1 \pp (S_2 \pp S_3)
	\end{array}
$$}
	\caption{Dynamic Correlation Calculus, structural congruence}
	\label{fig:jc_structural_congruence}
\end{figure}
