# Supplementary material for: Applied Choreographies
Source: arXiv:1510.03637 source file (2020-12-14)
Supplement: Supplementary file 2 [file compilation_example_supp.tex]

\begin{figure}[h]
%
%	ENCODING --- C
%
	\begin{displaymath}
		\overbrace{
		\jsrv{\genenc{\epp{C}{\pid f}}, \jprc{\genenc{\epp{C}{\pid c}}}{\env(\pid c).\estate}
		{\env( \pid c ).\equeues}}{l_\role C}}^{S_c}
		\quad \pp \quad
		\overbrace{
		\jsrv{\ \genenc{\epp{C}{\pid a}}, \inact}{l_\role A}}^{S_a}
		\quad \pp \quad
		\overbrace{
		\jsrv{\ \genenc{\epp{C}{\pid {dm}}}, \inact}{l_\role {DM}}}^{S_{dm}}
		\quad \pp \quad
		\overbrace{
		\jsrv{\ \genenc{\epp{C}{\pid l}}, \inact}{l_\role L}}^{S_l}
	\end{displaymath}
	% \caption{Parallel composition of the compiled services of
		% $\genenc{\env,\epp{C}{}}$}
  % \label{fig:example_compilation_services}
  \\
	\ResetLN
  {\footnotesize
  \begin{displaymath}
	{\setlength\arraycolsep{2pt}
	\genenc{\epp{C}{\pid c}} = \left\{
	\hspace{-3pt}\begin{array}{rl}
	\LN & \jpath{kd.C.l} = l_{\role C};
	\\
	\LN & \jpath{kd.A.l} = l_{\role A};
	\\
	\LN & \jpath{kd.DM.l} = l_{\role {DM}};
	\\
	\LN & \jpath{kd.L.l} = l_{\role L};
	\\
	% \LN & \ldots
	% \\
	% \LN & \jpath{kd.A.C} = \new;
	% \\
	\LN & \cq{\jpath{kd.A.C}};
	\\
	\LN & \notify{?}{\jpath{kd.A.l}}{\jpath{kd}};
	\\
	\LN & \oneway{sync}{\jpath{kd}} \qfrom{\jpath{kd.A.C}};
	\\
	% \LN & \jpath{kd.S.C} = \new;
	% \\
	% \LN & \cq{\jpath{kd.S.C}};
	\LN & \ldots
	\\
	% \LN & \notify{?}{\jpath{kd.S.l}}{\jpath{kd}};
	\LN & \ldots
	\\
	\LN & \notify{start}{\jpath{kd.A.l}}{\jpath{kd}} \qto{\jpath{kd.C.A}};
	\\
	\LN & \notify{start}{\jpath{kd.S.l}}{\jpath{kd}} \qto{\jpath{kd.C.S}};
	\\
	\LN & \notify{start}{\jpath{kd.C.l}}{\jpath{kd}} \qto{\jpath{kd.C.L}};
	\\
	\LN & \notify{get}{\jpath{kd.A.l}}{\m{mkReq()}} \qto{\jpath{kd.C.A}};
	\\
	\LN & \ldots
	\end{array}
	\right.
	% \\\\	
	% \jsrv{\inact, \jprc{\enc{\epp{C_{c}}{\pid c}}_{\pid c}}
	% 	{\env(\pid a).\estate}{\env(\pid a).\equeues}}{l_{\role C}}
	}
\qquad
%
%	ENCODING --- A
%
	\ResetLN
	{\setlength\arraycolsep{2pt}
	\genenc{\epp{C}{\pid a}} =
	\left\{
	\hspace{-3pt}\begin{array}{rl}
	\LN & \oneway{!}{\jpath{kd}};
	% \\
	% \LN & \jpath{kd.C.A} = \new;
	\\
	\LN & \cq{\jpath{kd.C.A}};
	% \\
	% \LN & \jpath{kd.S.A} = \new;
	\\
	\LN & \cq{\jpath{kd.S.A}};
	% \\
	% \LN & \jpath{kd.L.A} = \new;
	\\
	\LN & \cq{\jpath{kd.L.A}};
	\\
	\LN & \notify{sync}{\jpath{kd.C.l}}{\jpath{kd}} \qto{\jpath{kd.A.C}};
	\\
	\LN & \oneway{start}{\jpath{kd}} \qfrom{\jpath{kd.C.A}};
	\\
	\LN & \oneway{get}{\jpath{req}} \qfrom{\jpath{kd.C.A}};
	\\
	\LN & \cond{isValid( \jpath{req} ) }{
	\\ 
	\LN & \quad \notify{ok}{\jpath{kd.S.l}}{\jpath{req.rsc}} 
		\qto{\jpath{kd.A.S}};
	\\
	\LN & \quad \notify{ok}{\jpath{kd.C.l}}{} 
		\qto{\jpath{kd.A.C}}  
	\\ \LN & }{
	\\ 
	\LN & \quad \notify{ko}{\jpath{kd.S.l}}{\jpath{req.rsc}} 
		\qto{\jpath{kd.A.S}};
	\\
	\LN & \quad \notify{ko}{\jpath{kd.C.l}}{} 
		\qto{\jpath{kd.A.C}}  
	\\ \LN &
	}
	\end{array}
	\right.
	% \\\\	
	% \jsrv{\enc{\epp{C_{s}}{\pid a}}_{l_{\role A}} ,\inact}{l_{\role A}}
	}
  \end{displaymath}}
  \\
%
% ENCODING --- L
%
	\ResetLN
  {\footnotesize
  \begin{displaymath}
	{\setlength\arraycolsep{2pt}
	\genenc{\epp{C}{\pid l}} =
	\left\{
	\hspace{-2pt}\begin{array}{rl}
	\LN & \oneway{!}{\jpath{kd}};
	% \\
	% \LN & \jpath{kd.C.L}=\new;
	\\
	\LN & \cq{\jpath{kd.C.L}};
	% \\
	% \LN & \jpath{kd.A.L}=\new;
	\\
	\LN & \cq{\jpath{kd.A.L}};
	% \\
	% \LN & \jpath{kd.S.L}=\new;	
	\\
	\LN & \cq{\jpath{kd.S.L}};
	\\
	\LN & \notify{sync}{\jpath{k.C.l}}{\jpath{kd}} \qto{\jpath{kd.L.C}};
	\\
	\LN & \oneway{start}{\jpath{kd}} \qfrom{\jpath{kd.C.L}};
	\\
	\LN & \oneway{log}{\jpath{log}} \qfrom{\jpath{kd.S.L}}
	\end{array}
	\right.
	% \\\\
	% \jsrv{\enc{\epp{C_{s}}{\pid l}}_{l_{\role L}} ,\inact}{l_{\role L}}
	}
  \end{displaymath}}
	\hrule\mbox{}\\
	\caption{Compilation of $C = C_c \pp C_s$, from
	\cref{fig:choreography_example}. Compiled behaviour of
	processes $\pid {a}$, $\pid c$ (excepts) and $\pid l$.}
  \label{fig:example_compilation_full}
\end{figure}
